# Supplementary material for: Spin-current diode with a monoaxial chiral magnet
Source: arXiv:1903.12358 source file (2019-03-29)
Supplement: Supplementary file 1 [file Supplementary_Material.pdf]

# Supplementary Material for "Spin-current diode with a monoaxial chiral magnet"

Shun Okumura[1], Hiroaki Ishizuka[1], Yasuyuki Kato[1], Jun-ichiro Ohe[2], and Yukitoshi Motome[1]
[1]*Department of Applied Physics, the University of Tokyo, Tokyo 113-8656, Japan*
[2]*Department of Physics, Toho University, Chiba 274-8510, Japan*

## $J$ DEPENDENCE OF THE NONRECIPROCAL SPIN CURRENTS

In this section, we discuss the spin-charge coupling, $J$, dependence of the nonreciprocal spin currents. The results are qualitatively the same for different values of $J$ when $J$ is large enough so that the bands are split. We note that the sign of $\Delta G^z$ is reversed by changing the sign of $J$.

Figure S1 shows the results of the nonreciprocity as functions of $\varphi$ for different $J$ with a short period ($Q = 2\pi/3$). For $J = 2$, as shown in the main text, the nonreciprocity $\Delta G^\lambda$ is suppressed at small $|\varphi|$ and shows a peak at $|\varphi| \simeq 70^\circ$. As $J$ increases, the positions of the peaks of all the components of $\Delta G^\lambda$ shift to smaller $|\varphi|$. The result indicates that the region of $|\varphi|$ where the itinerant-electron spins can follow the localized spins is extended by increasing the spin-charge coupling. This supports our scenario discussed in the main text. This also implies that in the limit of $J \to \infty$, $\Delta G^\lambda$ will follow the related edge quantities, as in the case with a longer period in Fig. 4 in the main text. At the same time, however, the magnitude of the nonreciprocity approaches zero because the deviation of the itinerant-electron spins from the localized spins becomes small at the both edges of the sample. Such suppression while increasing $J$ is demonstrated in Fig. S1.

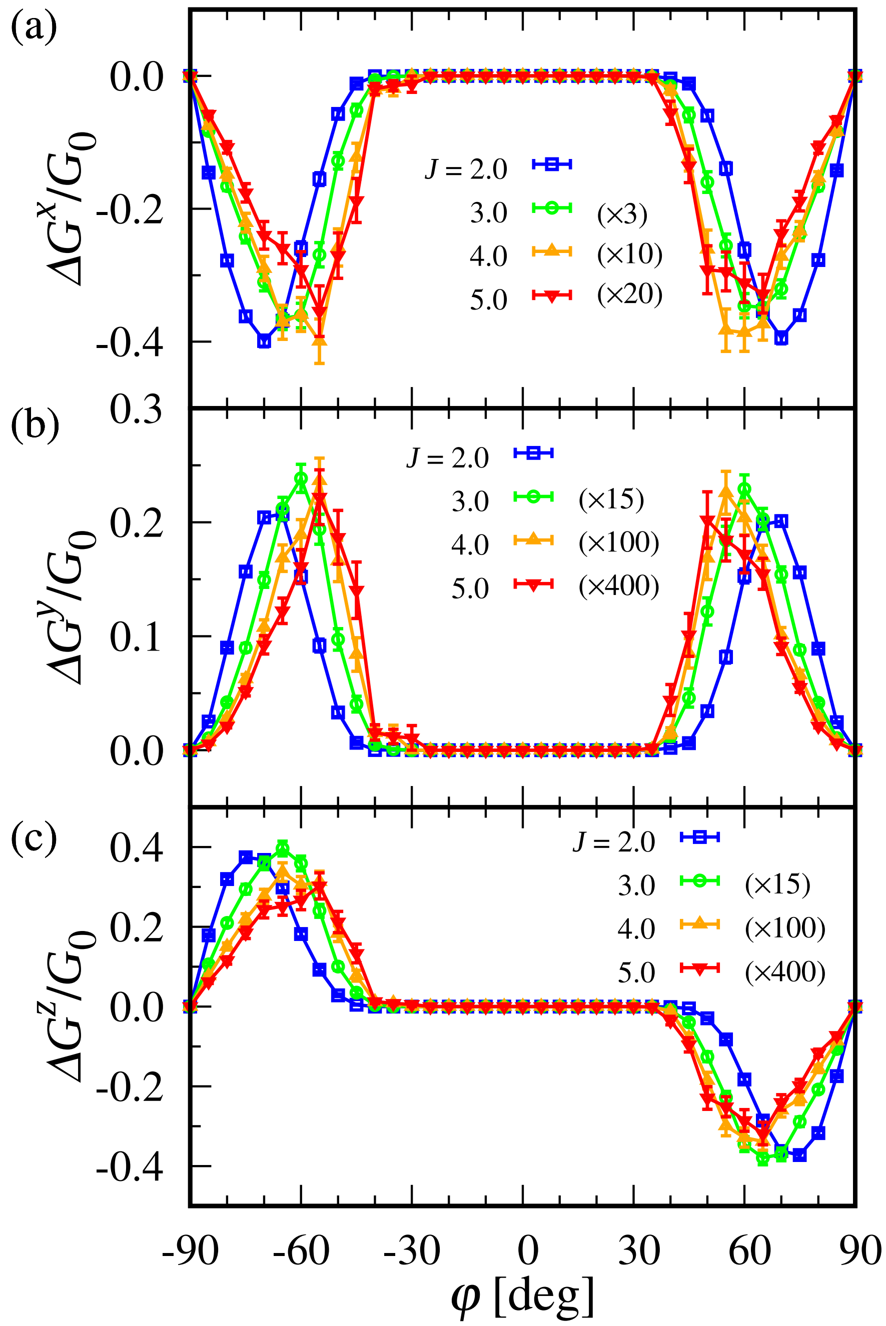


FIG. S1: Differences between the conductance of right- and left-going spin currents, $\Delta G^{\lambda}$, as functions of $\varphi$ for different $J$. We set the Fermi energy $\mu = 1.5 - J$ and the ordering vector $Q = 2\pi/3$ (right-handed chirality with a short period).
